# Supplementary material for: Continuous-Time Quantum Walks on Dynamic Graphs
Source: arXiv:1902.01346 source file (2019-02-04)
Supplement: Supplementary file 1 [file appendix.tex]

The following graphs show the probability of a system being in a quantum state with respect to time. We used the NDSolve method in Mathematica to generate the plots.
\begin{figure}[H]
\centering
\includegraphics[scale=0.5]{Test.png}
\caption{This is the X gate CTQW with the initial state $ \ket{0}$.}
\label{fig:xgraphone}
\end{figure}
%\begin{figure}[H]
%	\centering
%	\includegraphics[scale=0.75]{xgraphtwo.png}
%	\caption{This is the X gate CTQW with the initial state $ \sqrt{\frac{2}{3}} \ket{0} + \sqrt{\frac{1}{3}} \ket{1}$.}
%	\label{fig:xgraphtwo}
%\end{figure}
%%%%%%%%%%%%%%%
%\begin{figure}[H]
%	\centering
%	\includegraphics[scale=0.75]{xgraphthree.png}
%	\caption{This is the X gate CTQW with the initial state $ \sqrt{\frac{1}{2}} \ket{0} + \sqrt{\frac{1}{2}} \ket{1}$.}
%	\label{fig:xgraphthree}
%\end{figure}

%%%%%%%%%%%%%%
\begin{figure}[H]
	\centering
	\includegraphics[scale=.75]{zgraphone.png}
	\caption{This is the Z gate CTQW with the initial state $ \ket{000}$.}
	\label{fig:zgraphone}
\end{figure}
\begin{figure}[H]
	\centering
	\includegraphics[scale=.75]{zgraphtwo.png}
	\caption{This is the Z gate CTQW with the initial state $ \sqrt{\frac{1}{3}} \ket{000} + \sqrt{\frac{2}{3}} \ket{001}$.}
	\label{fig:zgraphtwo}
\end{figure}
\begin{figure}[H]
	\centering
	\includegraphics[scale=.75]{zgraphthree.png}
	\caption{This is the Z gate CTQW with the initial state $ \sqrt{\frac{1}{2}} \ket{000} + \sqrt{\frac{1}{2}} \ket{001}$.}
	\label{fig:zgraphthree}
\end{figure}
%%%%%%%%%%
\begin{figure}[H]
	\centering
	\includegraphics[scale=.75]{ygraphone.png}
	\caption{This is the Y gate CTQW with the initial state $ \ket{000}$.}
	\label{fig:ygraphone}
\end{figure}
\begin{figure}[H]
	\centering
	\includegraphics[scale=.75]{ygraphtwo.png}
	\caption{This is the Y gate CTQW with the initial state $ \sqrt{\frac{1}{3}} \ket{000} + \sqrt{\frac{2}{3}} \ket{001}$.}
	\label{fig:ygraphtwo}
\end{figure}
\begin{figure}[H]
	\centering
	\includegraphics[scale=.75]{ygraphthree.png}
	\caption{This is the Y gate CTQW with the initial state $ \sqrt{\frac{1}{2}} \ket{000} + \sqrt{\frac{1}{2}} \ket{001}$.}
	\label{fig:ygraphthree}
\end{figure}
\begin{figure}[H]
	\centering
	\includegraphics[scale=.75]{hgraphone.png}
	\caption{This is the Hadamard gate CTQW with the initial state $\ket{0}$.}
	\label{fig:hgraphone}
\end{figure}
\begin{figure}[H]
	\centering
	\includegraphics[scale=.75]{hgraphtwo.png}
	\caption{This is the Hadamard gate CTQW with the initial state $ \sqrt{\frac{1}{3}} \ket{0} + \sqrt{\frac{2}{3}} \ket{1}$.}
	\label{fig:hgraphtwo}
\end{figure}
\begin{figure}[H]
	\centering
	\includegraphics[scale=.75]{hgraphthree.png}
	\caption{This is the Hadamard gate CTQW with the initial state $ \sqrt{\frac{1}{2}} \ket{0} + \sqrt{\frac{1}{2}} \ket{1}$.}
	\label{fig:hgraphthree}
\end{figure}

\begin{figure}[H]
	\centering
	\includegraphics[scale=0.75]{tgraphone.png}
	\caption{This is the $T$ gate CTQW with the initial state $ \ket{000}$.}
	\label{fig:tgraphone.png}
\end{figure}
\begin{figure}[H]
	\centering
	\includegraphics[scale=0.75]{tgraphtwo.png}
	\caption{This is the $T$ gate CTQW with the initial state $ \sqrt{\frac{1}{3}} \ket{000} + \sqrt{\frac{2}{3}} \ket{001}$.}
	\label{fig:tgraphtwo.png}
\end{figure}
%%%%%%%%%%%%%%
\begin{figure}[H]
	\centering
	\includegraphics[scale=0.75]{tgraphthree.png}
	\caption{This is the $T$ gate CTQW with the initial state $ \sqrt{\frac{1}{2}} \ket{000} + \sqrt{\frac{1}{2}} \ket{001}$.}
	\label{fig:tgraphthree.png}
\end{figure}
\begin{figure}[H]
	\centering
	\includegraphics[scale=0.75]{cxgraphone.png}
	\caption{This is the CNOT gate CTQW with the initial state $ \ket{10}$.}
	\label{fig:cxgraphone.png}
\end{figure}
\begin{figure}[H]
	\centering
	\includegraphics[scale=0.75]{cxgraphtwo.png}
	\caption{This is the CX gate CTQW with the initial state $ \sqrt{\frac{1}{3}} \ket{10} + \sqrt{\frac{2}{3}} \ket{11}$.}
	\label{fig:cxgraphtwo.png}
\end{figure}
\begin{figure}[H]
	\centering
	\includegraphics[scale=0.75]{cxgraphthree.png}
	\caption{This is the CX gate CTQW with the initial state $ \sqrt{\frac{1}{2}} \ket{10} + \sqrt{\frac{1}{2}} \ket{11}$.}
	\label{fig:cxgraphthree.png}
\end{figure}
\begin{figure}[H]
	\centering
	\includegraphics[scale=0.75]{toffgraphone.png}
	\caption{This is the Toffoli gate CTQW with the initial state $ \ket{111}$.}
	\label{fig:toffgraphone.png}
\end{figure}
\begin{figure}[H]
	\centering
	\includegraphics[scale=0.75]{toffgraphtwo.png}
	\caption{This is the Toffoli gate CTQW with the initial state $ \sqrt{\frac{1}{3}} \ket{110} + \sqrt{\frac{2}{3}} \ket{111}$.}
	\label{fig:toffgraphtwo.png}
\end{figure}
%%%%%%%%%%%%%%
\begin{figure}[H]
	\centering
	\includegraphics[scale=0.75]{toffgraphthree.png}
	\caption{This is the Toffoli gate CTQW with the initial state $ \sqrt{\frac{1}{2}} \ket{110} + \sqrt{\frac{1}{2}} \ket{111}$.}
	\label{fig:toffgraphthree.png}
\end{figure}
%\begin{figure}[H]
%	\centering
%	\includegraphics[scale=.75]{ugraphone.png}
%	\caption{This is the qubit rotation CTQW to the state % $\ket{1}$.}
%	\label{fig:qrgraphone}
%\end{figure}
%\begin{figure}[H]
%	\centering
%	\includegraphics[scale=.75]{ugraphtwo.png}
%	\caption{This is the qubit rotation CTQW to the state $ \sqrt{\frac{1}{3}} \ket{0} + \sqrt{\frac{2}{3}} \ket{1}$.}
%	\label{fig:qrgraphtwo}
%\end{figure}
%\begin{figure}[H]
%	\centering
%	\includegraphics[scale=.75]{ugraphthree.png}
%	\caption{This is the qubit rotation CTQW to the state $ \sqrt{\frac{1}{2}} \ket{0} + \sqrt{\frac{1}{2}} \ket{1}$.}
%	\label{fig:qrgraphthree}
%\end{figure}
